# Supplementary material for: Conformational Entropy as Collective Variable for Proteins
Source: arXiv:1704.03344 ancillary file (2017-04-10)
Supplement: Supplementary file 1 [file SuppMat_PalazzesiValssonParrinello.pdf]

# Supplemental Material for "Conformational Entropy as Collective Variable for Proteins"

Ferruccio Palazzesi,[1] Omar Valsson,[1,2] and Michele Parrinello[1,2,*]

[1]*Department of Chemistry and Applied Biosciences, ETH Zurich and Facoltà di Informatica, Instituto di Scienze Computationali, Università della Svizzera italiana, Via Giuseppe Buffi 13, CH-6900, Lugano, Switzerland.*
[2]*National Center for Computational Design and Discovery of Novel Materials MARVEL.*

## Variationally Enhanced Sampling Simulations for Chignolin

In VES sampling is expedited by constructing a bias V(s) that is obtained by minimizing the convex functional $\Omega[V]$ [1]:

$$\Omega[V] = \frac{1}{\beta} \log \frac{\int d\mathbf{s}\, e^{-\beta[F(\mathbf{s})+V(\mathbf{s})]}}{\int d\mathbf{s}\, e^{-\beta F(\mathbf{s})}} + \int d\mathbf{s}\, p(\mathbf{s}) V(\mathbf{s}), \tag{1}$$

where $p(\mathbf{s})$ is a target probability distribution.

The free energy surface $F(\mathbf{s})$ can be obtained from the bias that minimizes $\Omega[V]$ as

$$F(\mathbf{s}) = -V(\mathbf{s}) - \frac{1}{\beta} \log p(\mathbf{s}). \tag{2}$$

The $p(\mathbf{s})$ will determine the distribution of $\mathbf{s}$ in the biased ensemble. In our case we write $p(\mathbf{s})$ as a linear combination of two bivariate Gaussians distributions that are centered on the folded and unfolded state:

$$p(\mathbf{s}) = w_f\, p_{b,f}(\mathbf{s}) + w_u\, p_{b,u}(\mathbf{s}), \tag{3}$$

where $w_f$ and $w_u$ are the weights of the folded and unfolded state, respectively. Each bivariate Gaussians distribution is given by

$$p_b(\mathbf{s}) = \frac{A}{2\pi\sigma_{s_S}\sigma_{s_H}\sqrt{1-\rho^2}} \exp\left[ -\frac{1}{2(1-\rho^2)} \left( \left(\frac{s_S-\mu_S}{\sigma_S}\right)^2 + \left(\frac{s_H-\mu_H}{\sigma_H}\right)^2 - 2\rho \left(\frac{s_S-\mu_S}{\sigma_S}\right)\left(\frac{s_H-\mu_S}{\sigma_H}\right)\right)\right], \tag{4}$$

where $\rho$ is the correlation between the two CVs $s_S$ and $s_H$, and $\mu$ and $\sigma$ are the mean and sigma used for the CVs, respectively. $A$ is normalization factor that can be used to ensure that the distribution is properly normalized to 1 over the region on which the bias is defined. The parameters for the bivariate Gaussians are obtained by performing two separate unbiased runs in the folded and unfolded state and measuring the expectation values and fluctuations of the CVs. Since we calculate the fluctuations from unbiased runs of limited time we are likely to underestimate them. To account for this, we employ slightly higher values for the $\sigma$ than these estimated from the unbiased runs. For the distribution $p_{b,f}(\mathbf{s})$ corresponding to the folded state we use $\mu_{s_S}$=2.9, $\sigma_{s_S}$=0.25, $\mu_{s_H}$=2.6, $\sigma_{s_H}$=0.25, and $\rho = 0$ (uncorrelated CVs). For the distribution $p_{b,u}(\mathbf{s})$ corresponding to the the unfolded state we employ $\mu_{s_S}$=1.4, $\sigma_{s_S}$=0.6, $\mu_{s_H}$=0.1, $\sigma_{s_H}$=0.3, and $\rho = 0.5$. The weights are taken as $w_f = 2/3$ and $w_u = 1/3$ such that the folded state is favored in the target distribution. To ensure that there are not barriers in-between the folded and unfolded state in target distribution do we furthermore transform it as:

$$p(s) \rightarrow \frac{p(s)^{1/\gamma}}{\int ds\, p(s)^{1/\gamma}}, \tag{5}$$

by using a value of $\gamma$ equivalent to 2. The final target distribution employed in the simulation is shown in Fig. 1.

The bias potential is expanded in a linear expansion of a product of Legendre polynomials

$$V(\mathbf{s}, \boldsymbol{\alpha}) = \sum_{k_S,k_H} \alpha_{k_S,k_H}\, P_{k_S}(\tilde{s}_S)\, P_{k_H}(\tilde{s}_H), \tag{6}$$

where $\tilde{s}_S$ and $\tilde{s}_H$ are the values of the CVs after being translated from the interval on which the bias is defined to the interval -1 to 1 on which the Legendre polynomials are naturally defined. For $s_S$ we employ 20 Legendre polynomials in the expansion and take them to be on the interval from 0.0 to 4.0. For $s_H$ we employ 40 Legendre polynomials in the expansion and take them to be on the interval from 0.5 to 3.5.

The expansion coefficients $\alpha_{k_S,k_H}$ are optimized using the procedure introduced in Ref. 1. We employ the averaged stochastic gradient decent from Ref. 2 and update the coefficient every 4 ps and employ a fixed step size of 0.1. The optimization is performed using 4 multiple walkers.

In Fig. 2 we report the reweighted FES as a function of enthalpy and entropy from the VES simulation.

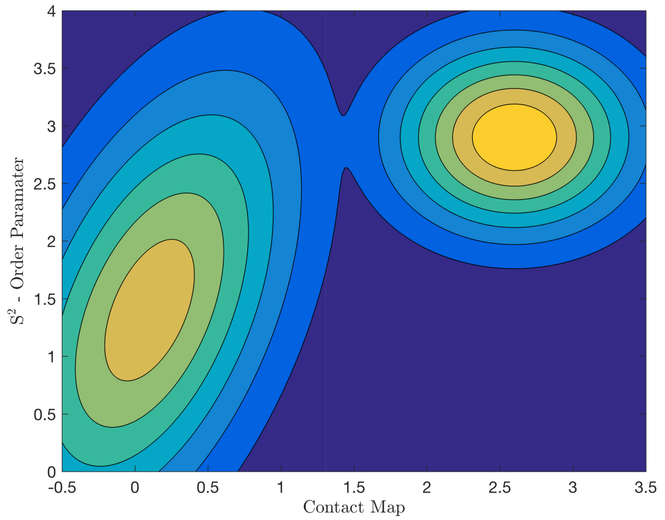


FIG. 1. Target distribution $p(\mathbf{s})$ employed in the VES simulation for chignolin.

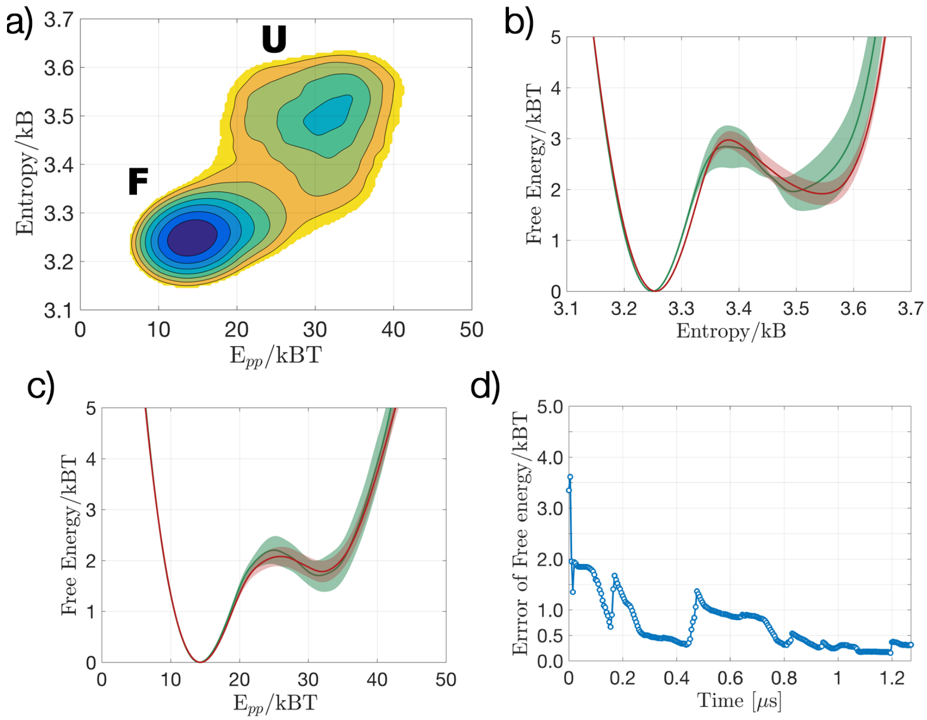


FIG. 2. a) Reweighted FES calculated from the VES simulation using entropy and enthalpy as CVs. b) and c) Mono-dimensional entropy and enthalpy FES. In red the data from the unbiased simulation of Ref. 3, while in green the one from VES simulation. d) Free energy error calculated from the 2D FES, along the simulation time. This value is calculated using the error metric previously used in Ref. [4–6] and using the unbiased data of Ref. 3 as reference.

## Unfolding Times of Chignolin

For the calculation of the unfolding time we make use of the approach reported in Ref. 7. Thus we first optimize the VES bias at 340 K using $s_S$ as biasing CV, with a free energy cutoff of 9 kJ/mol to assure that the transition region

is not corrupted by the bias. The bias potential is expanded linearly in a series of 40 Chebyshev polynomials that are defined in the interval from 1.5 to 3. For the optimization (see above) we update the coefficient every 4 ps and employ a step size of 0.01. The optimization is performed using 4 multiple walkers.

We then run 25 independent molecular dynamics simulations using the optimized bias as external potential to facilitate the unfolding of the systems. The unbiased unfolding times are then obtained using

$$t_{\text{unbiased}} = t_{\text{biased}} \langle e^{(\beta V(s))} \rangle_V \tag{7}$$

where $\langle e^{(\beta V(s))} \rangle_V$ is an average obtained in the biased simulation. This average is often called the acceleration factor as tells how much the simulation is speed up by the bias potential. In order to check the validity of the assumption that we are simulating a rare event and that we did not corrupt the transition state with the bias we employ the Kolmogorov-Smirnov test from Ref. 8. We furthermore repeated our simulations using a smaller free energy cutoff of 8 kJ/mol and obtained a similar unfolding time.

To obtain the unfolding simulations at the lower temperatures 320 K and 300 K we did not optimize again the VES bias with an higher free-energy cutoff. Rather we employed the bias potential obtained at 340 K using a free energy cutoff of 9 kJ/mol. This is possible as we are only slightly decreasing the temperature which will only increase the barrier height. Due to the increased barrier height we also employ infrequent metadynamics [9] to speed up the unfolding process. For the infrequent metadynamics we deposit Gaussian hills every 300 ps, employ a height equal to 0.5 kJ/mol, a sigma of 0.02, and a bias factor of 5.

* parrinello@phys.chem.ethz.ch

[1] O. Valsson and M. Parrinello, Phys. Rev. Lett. **113**, 090601 (2014).
[2] F. Bach and E. Moulines, in *Advances in Neural Information Processing Systems 26*, edited by C. Burges, L. Bottou, M. Welling, Z. Ghahramani, and K. Weinberger (Curran Associates, Inc., Red Hook, NY, 2013) pp. 773–781.
[3] K. Lindorff-Larsen, S. Piana, R. O. Dror, and D. E. Shaw, Science **334**, 517 (2011).
[4] A. Barducci, G. Bussi, and M. Parrinello, Phys. Rev. Lett. **100**, 020603 (2008).
[5] D. Branduardi, G. Bussi, and M. Parrinello, J. Chem. Theory Comput. **8**, 2247 (2012).
[6] O. Valsson and M. Parrinello, Journal of chemical theory and computation **11**, 1996 (2015).
[7] J. McCarty, O. Valsson, P. Tiwary, and M. Parrinello, Phys. Rev. Lett. **115**, 070601 (2015).
[8] M. Salvalaglio, P. Tiwary, and M. Parrinello, J. Chem. Theory Comput. **10**, 1420 (2014).
[9] P. Tiwary and M. Parrinello, Physical review letters **111**, 230602 (2013).
